# Supplementary material for: Selective nonlinearities removal from digital signals
Source: arXiv:2403.09731 source file (2024-03-13)
Supplement: Supplementary file 1 [file X_suppl.tex]

\clearpage
\setcounter{page}{1}
\maketitlesupplementary

\appendix
\section{Hyperparameter tuning}
\label{appendix:hyperparameter_tuning}

\begin{table}
  \centering
  \begin{tabular}{@{}lc@{}l}
    \toprule
    Parameter& Values &\\
    \midrule
    Theirs & Frumpy  &\\
    Yours & Frobbly  &\\
    Ours & Makes one's heart Frob &\\
    \bottomrule
  \end{tabular}
  \caption{Results.   Ours is better.}
  \label{tab:hyperparameters}
\end{table}

Having the supplementary compiled together with the main paper means that:
\begin{itemize}
\item The supplementary can back-reference sections of the main paper, for example, we can refer to \cref{sec:intro};
\item The main paper can forward reference sub-sections within the supplementary explicitly (e.g. referring to a particular experiment); 
\item When submitted to arXiv, the supplementary will already included at the end of the paper.
\end{itemize}
To split the supplementary pages from the main paper, you can use \href{https://support.apple.com/en-ca/guide/preview/prvw11793/mac#:~:text=Delete%20a%20page%20from%20a,or%20choose%20Edit%20%3E%20Delete).}{Preview (on macOS)}, \href{https://www.adobe.com/acrobat/how-to/delete-pages-from-pdf.html#:~:text=Choose%20%E2%80%9CTools%E2%80%9D%20%3E%20%E2%80%9COrganize,or%20pages%20from%20the%20file.}{Adobe Acrobat} (on all OSs), as well as \href{https://superuser.com/questions/517986/is-it-possible-to-delete-some-pages-of-a-pdf-document}{command line tools}.
